# Supplementary material for: Converged Colored Noise Path Integral Molecular Dynamics Study of the Zundel Cation down to Ultra-low Temperatures at Coupled Cluster Accuracy
Source: arXiv:2103.13063 ancillary file (2021-03-24)
Supplement: Supplementary file 1 [file si.pdf]

# Supporting Information:

# Converged Colored Noise Path Integral Molecular Dynamics Study of the Zundel Cation down to Ultra-low Temperatures at Coupled Cluster Accuracy


Christoph Schran,[1] Fabien Brieuc,[1] and Dominik Marx[1]

[1] *Lehrstuhl für Theoretische Chemie, Ruhr-Universität Bochum, 44780 Bochum, Germany*


## I. PATH INTEGRAL QUANTUM THERMAL BATH (PIQTB)

### A. Basics of the method

Let us consider the simple case of a one dimensional harmonic oscillator of angular frequency $\omega$ and mass $m$. In the path integral framework, all properties as given by the respective quantum expectation values converge to their exact quantum values in the limit of infinite number of Trotter replicas $P$. In particular, the average total energy of the harmonic oscillator,

$$\lim_{P\to\infty} \langle E(\omega)\rangle_P = \frac{\hbar\omega}{2} \coth\left(\frac{\beta\hbar\omega}{2}\right), \tag{1}$$

is exactly recovered in that limit. The main idea of the Path Integral Quantum Thermal Bath method, PIQTB, is to use the quantum thermal bath method [1] to impose this exact quantum energy for any value of $P$. This is achieved, in practice, by applying the QTB on the normal modes of the ring polymer with a modified random force whose power spectrum now depends on the number of beads used in the simulation [2]. Indeed, one can transform the bead coordinates $q_s$ $(s = 1, ..., P)$ to the ring polymer normal mode coordinates $\tilde{q}_k$ $(k = 1, ..., P)$ using a normal mode transformation defined as

$$\tilde{q}_k = \sum_{k=1}^{P} q_s C_{sk} \tag{2}$$

with the well-known elements $C_{sk}$ of the transformation matrix being given, for instance, in the Appendix of Ref. 2. The normal modes obtained are uncoupled harmonic oscillators of angular frequencies $\omega_k$ given by

$$\omega_k = \sqrt{\omega^2 + 4\,\omega_P^2 \sin^2\left((k-1)\pi/P\right)}. \tag{3}$$

One can show that, in the harmonic case, the position fluctuations of the beads and the normal modes are related by

$$\langle q_s^2\rangle = \frac{1}{P}\sum_{k=1}^{P}\langle \tilde{q}_k^2\rangle \qquad \forall s = 1, ..., P. \tag{4}$$

In our harmonic case, the position fluctuations are connected to the average total energy in the following way,

$$\langle q_s^2\rangle = \frac{1}{m\omega^2}\langle E(\omega)\rangle_P, \quad \langle \tilde{q}_k^2\rangle = \frac{1}{m\omega_k^2}\langle \tilde{E}(\omega_k)\rangle_P, \tag{5}$$

with $\langle \tilde{E}(\omega_k)\rangle_P$ being the average total energy of the $k$-th normal mode and $\langle E(\omega)\rangle_P$ the average total energy of the harmonic oscillator that can be expressed as given in the main text,

$$\langle E(\omega)\rangle_P = \frac{1}{P}\sum_{k=1}^{P}\frac{\omega^2}{\omega_k^2}\langle \tilde{E}(\omega_k)\rangle_P, \tag{6}$$

by introducing Eqs. (5) in Eq. (4). In the standard PIMD case, the ring polymer is classically thermalized at the temperature $T \times P$, so that $\langle \tilde{E}(\omega_k)\rangle_P = k_{\mathrm{B}}T \times P$. When the number of replicas $P$ increases, the average energy of the

harmonic oscillator converges towards its exact quantum value. As already explained, the main idea of the PIQTB method is to use the QTB to ensure that $\langle E(\omega)\rangle_P$ is given by the exact quantum expression for any value of $P$ for the harmonic oscillator. In order to do this, we need to enforce an energy distribution $\langle \tilde{E}(\omega_k)\rangle_P$ among the ring polymer normal modes that is solution of the following equation,

$$\frac{1}{P}\sum_{k=1}^{P}\frac{\omega^2}{\omega_k^2}\langle \tilde{E}(\omega_k)\rangle_P = \frac{\hbar\omega}{2}\coth\left(\frac{\beta\hbar\omega}{2}\right), \tag{7}$$

which is directly obtained by combining Eqs. (1) and (6). This equation can be solved numerically for any value of $P$ and the obtained energy distribution $\langle \tilde{E}(\omega_k)\rangle_P$ can then be enforced by applying the QTB to the normal modes with a random force whose power spectrum is directly proportional to $\langle \tilde{E}(\omega_k)\rangle_P$ as shown earlier [2].

All this is exact for the harmonic oscillator, but when applied to a realistic (*i.e.* anharmonic interacting many-body) system this method is able to include a large part of the quantum fluctuations via the thermostat so that the number of replicas required to converge the simulation gets significantly reduced. We close by recalling that the PIQTB method is closely related to the Path Integral Generalized Langevin Equation Thermostat (PIGLET) approach [3] introduced earlier, which is based in its turn on the Generalized Langevin Equation (GLE) thermostat [4], as explained in the Sec. II of the main text.

### B. Kinetic Energy Estimator

Several estimators used in PIMD assume that the beads are classically thermalized, as it is the case in standard PIMD in the limit that sampling is ergodic. This is not true anymore when employing colored noise thermostats (so for both PIGLET and PIQTB) which requires special care when computing energies. For instance, the usual centroid virial estimator usually used to compute the average kinetic energy,

$$\langle K\rangle = \frac{3N}{2\beta} + \frac{1}{2P}\sum_{i=1}^{N}\sum_{s=1}^{P}\left\langle\left(\mathbf{q}_{i,s}-\mathbf{q}_{i,c}\right)\cdot\nabla_s V\left(\mathbf{q}_s\right)\right\rangle, \tag{8}$$

assumes that the centroid of the ring polymer, defined as $\mathbf{q}_{i,c} = \sum_{s=1}^{P}\mathbf{q}_{i,s}/P$, is a classical variable. Indeed, if we apply this estimator to our previous case of the 1D harmonic oscillator we obtain the following expression,

$$\langle K\rangle = \frac{1}{2\beta} - \left\langle \frac{1}{2}m\omega^2 q_c^2\right\rangle + \langle V\rangle, \tag{9}$$

where we see that the average kinetic and potential energies are only equal (which is neccessary for a harmonic oscillator) if the centroid is classical [3]. Indeed, the first term in the centroid virial estimator in Eq. (8) is the classical expression for the average kinetic energy of the centroid.

This problem can be solved by modifying the estimator replacing the first term by the actual expression of the centroid kinetic energy [2] so that the modified centroid virial estimator is given by

$$\langle K\rangle = \sum_{i=1}^{N}\frac{\mathbf{p}_{i,c}^2}{2m_i} + \frac{1}{2P}\sum_{s=1}^{P}\left\langle\left(\mathbf{q}_s-\mathbf{q}_c\right)\cdot\nabla_s V\left(\mathbf{q}_s\right)\right\rangle. \tag{10}$$

Note that the expression here is slightly different from that given in Ref. 2 because we use here a different (although equivalent) formulation of PIMD where each bead is submitted to the physical potential and the simulation temperature is $T\times P$. One can also decide to ensure that the centroid is classically distributed by coupling the centroid normal mode ($k=1$) to a classical thermostat while the other modes ($k=2,..,P$) remain coupled to the colored noise thermostat. This solution allows one to continue using the standard centroid virial estimator and requires to impose that $\langle \tilde{E}(\omega_1)\rangle_P = k_{\rm B}T\times P$ in Eq. (7). This is the procedure used in the PIGLET thermostat [3], where the centroid normal mode is classically thermalized and the other normal modes are coupled to a GLE thermostat enforcing the quantum fluctuations. In our PIQTB simulations reported herein, we also used this procedure so that the centroid normal mode is coupled to a classical Langevin thermostat and the other modes are submitted to the QTB random forces. This procedure is equivalent to the formulation using the $f_P^{(1)}$ function in the original publication [2]. However, if strong anharmonic couplings between the normal modes are present, zero-point energy leakage (ZPEL) can lead to a transfer of energy from the high frequency modes to the centroid mode, which would then have an average energy higher than the expected classical value. In this case, the standard centroid virial estimator would again not be adapted and one should still use the modified expression of Eq. (10). Thus, in our PIQTB simulations, the average kinetic energies are computed using the modified centroid virial estimator.

### C. Implementation of PIQTB in CP2k

We have implemented the PIQTB method as described in the previous sections in the `CP2k` simulation package [5, 6]. Our implementation is based on the PILE thermostat [7] where each ring polymer normal mode is coupled to a Langevin thermostat with a friction coefficient adapted to its normal mode angular frequency. In the PILE thermostat, the friction coefficient of the thermostat attached to the centroid normal mode ($k = 1$) is $\gamma_1 = 1/\tau$ whereas the friction coefficients associated to the other normal modes ($k \geq 2$) are given by $\gamma_k = \tilde{\omega}_k$ where $\tilde{\omega}_k$ are the angular frequencies of the free ring polymer normal modes (a.k.a. Matsubara frequencies) given by $\tilde{\omega}_k = 2\omega_P \sin((k-1)\pi/P)$.

The standard QTB method introduces two parameters: a friction coefficient $\gamma$ (as in the standard Langevin thermostat) and an angular frequency cutoff $\omega_{\rm cut}$ for the generation of the random forces [8]. In order to correctly choose the values of these coefficients one needs to approximately know the range of the physical vibration frequencies $[\omega_{\rm min}, \omega_{\rm max}]$ of the system under study. A standard and reasonable choice [8] for the angular cutoff frequency is $\omega_{\rm cut} \approx 2\ \omega_{\rm max}$. The value of the friction coefficient $\gamma$ is a little more complicated to choose. On one hand, the value of $\gamma$ should be small enough to avoid any divergence of the kinetic energy. For a harmonic oscillator of angular frequency $\omega$ and using a cutoff frequency $\omega_{\rm cut} \approx 2\omega_{\rm max}$ one finds that a value around $\gamma/\omega \approx 0.05$ ensures that there is absolutely no divergence [8]. On the other hand, increasing $\gamma$ is able to strongly reduce the effect of ZPEL in anharmonic systems. Thus, in practice, the best way to optimally choose the value of the friction coefficient is to start from a rather small value compared to the typical frequencies of the system and then to increase $\gamma$ as much as possible while checking that no significant divergence of the kinetic energy appears. In the same spirit as in the PILE thermostat, every ring polymer normal mode is coupled to its own thermostat in our PIQTB implementation. The centroid normal mode ($k = 1$) can be coupled to a QTB thermostat or a classical Langevin thermostat (corresponding respectively to the formulation with function $f_P^{(0)}$ or $f_P^{(1)}$ in the original PIQTB publication [2]). The other normal modes ($k \geq 2$) are finally attached to QTB thermostats. The friction coefficient values are scaled according to the angular frequency of the normal modes so that the friction coefficient associated with normal mode $k$ is given by

$$\gamma_k = \sqrt{(1/\tau)^2 + \lambda^2\, \tilde{\omega}_k^2}. \qquad (11)$$

In the same way, the cutoff angular frequencies are given by

$$\omega_{{\rm cut},k} = \sqrt{(1/\tau_{\rm cut})^2 + \lambda_{\rm cut}^2\, \tilde{\omega}_k^2}. \qquad (12)$$

In conclusion, the only parameters that need to be specified in the PIQTB input in our implementation in `CP2k` are $\tau$, $\tau_{\rm cut}$, $\lambda$ and $\lambda_{\rm cut}$. For the Zundel cation, we found that $\tau = 50$ fs, $\tau_{\rm cut} = 0.9$ fs, $\lambda = 0.2$ and $\lambda_{\rm cut} = 1.5$ are rather satisfactory values.

Finally, we note that the random forces are generated on the fly as introduced earlier [8] which introduces one additional parameter, being the number of points used to discretize the target power spectrum of the random forces, $N_{\rm f}$. The value of $N_{\rm f}$ can also be given as an input in our implementation, however the default value ($N_{\rm f} = 100$) selected in `CP2k` is generally able to give satisfactory results.

## II. SUPPORTING ANALYSIS ON STRUCTURAL PROPERTIES

In the following, we provide complementary figures showing the convergence of the structural properties discussed in detail in the main text in Sec. IV.B without further discussion. In particular, these figures display the underlying distribution functions of Fig. 2 in the main text.

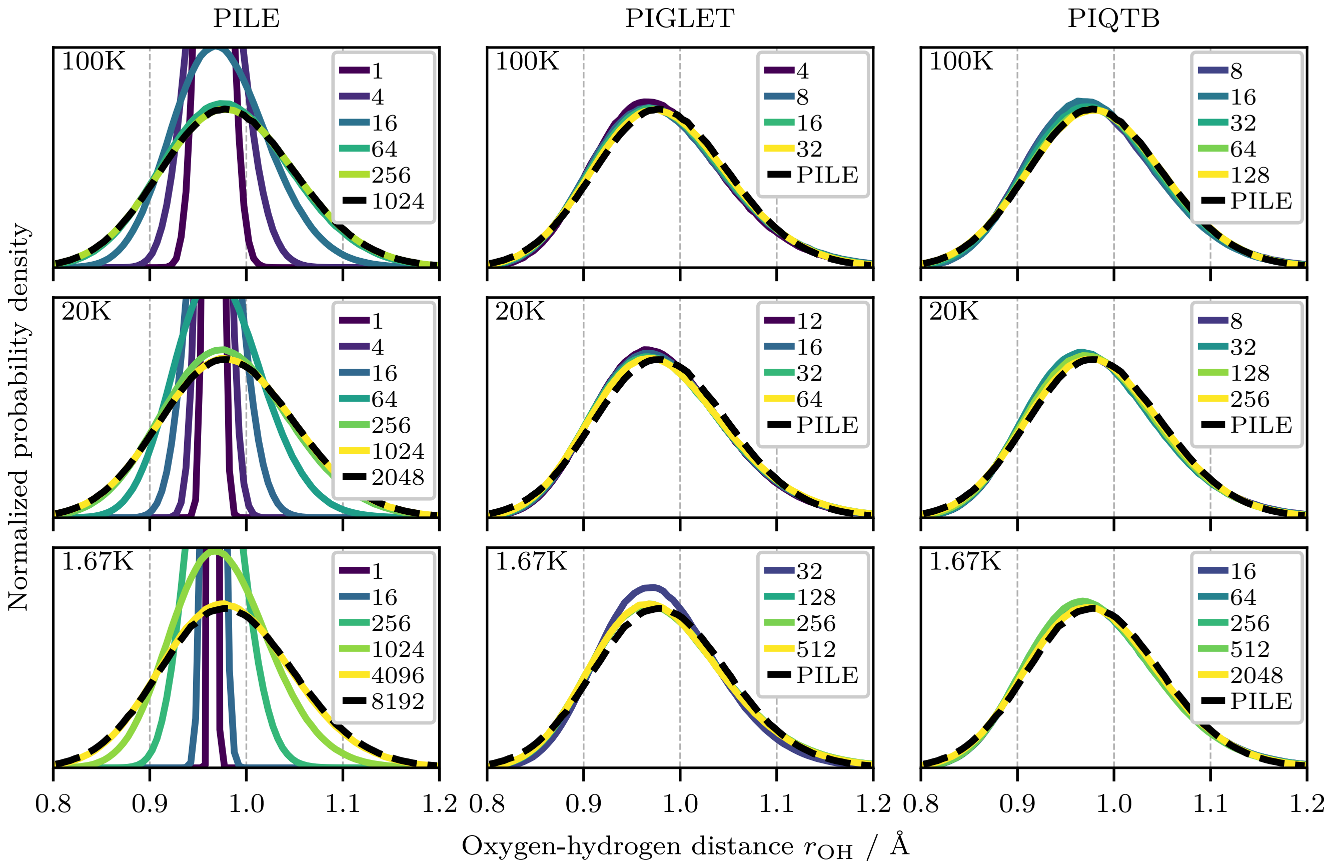


Figure 1. Distribution functions of the oxygen-hydrogen distance between the dangling hydrogen atoms and their closest oxygen atom, $r_{\mathrm{OH}}$, for different numbers of replicas $P$ at $T$ =100, 20 and 1.67 K for the PILE (left), PIGLET (middle) and PIQTB (right) thermostats (where in the middle and right panels the dashed black lines correspond to the PILE reference data obtained with the largest $P$ value).

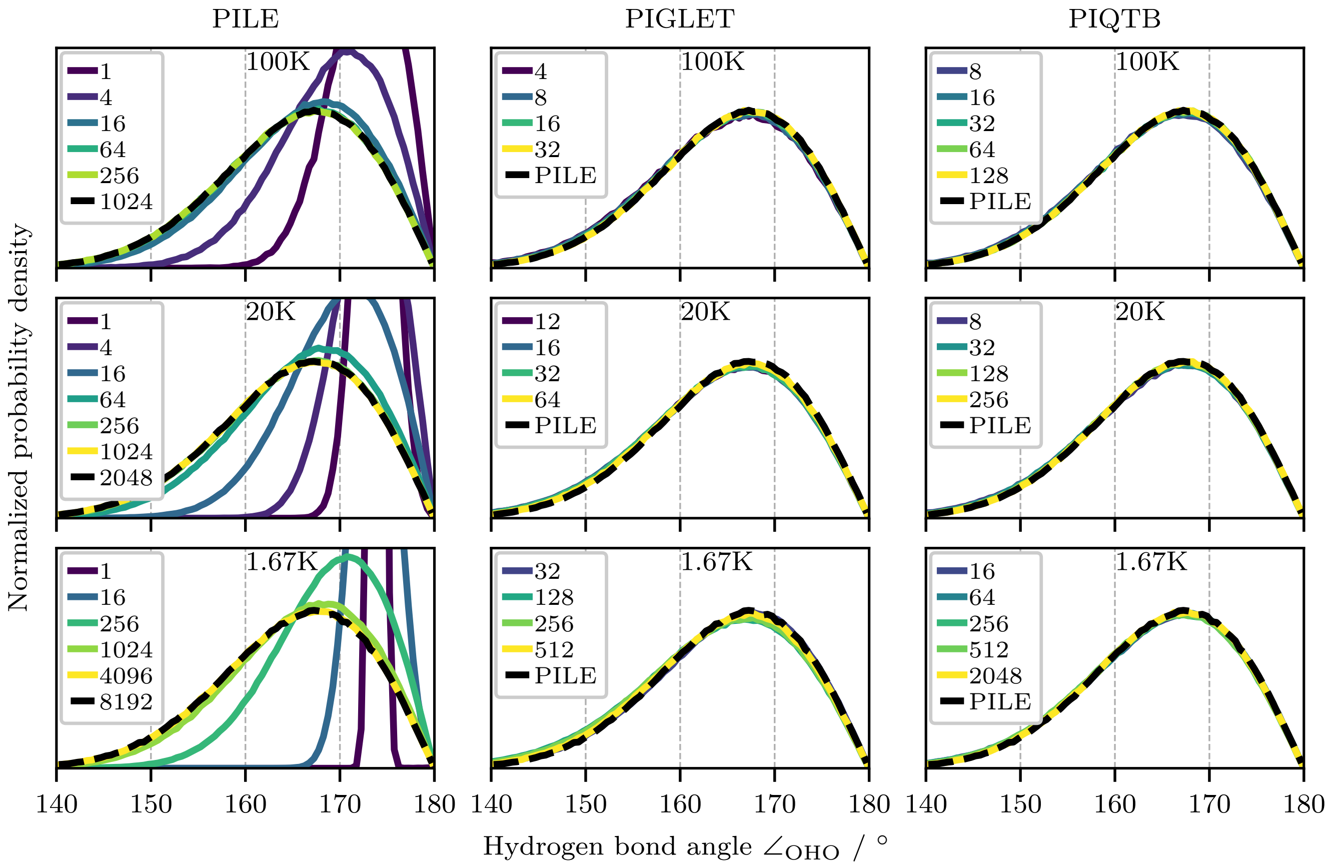


Figure 2. Distribution functions of the hydrogen bond angle between the shared proton and the two oxygen atoms, $\angle_{\mathrm{OHO}}$, for different numbers of replicas $P$ at $T$ =100, 20 and 1.67 K for the PILE (left), PIGLET (middle) and PIQTB (right) thermostats (where in the middle and right panels the dashed black lines correspond to the PILE reference data obtained with the largest $P$ value).

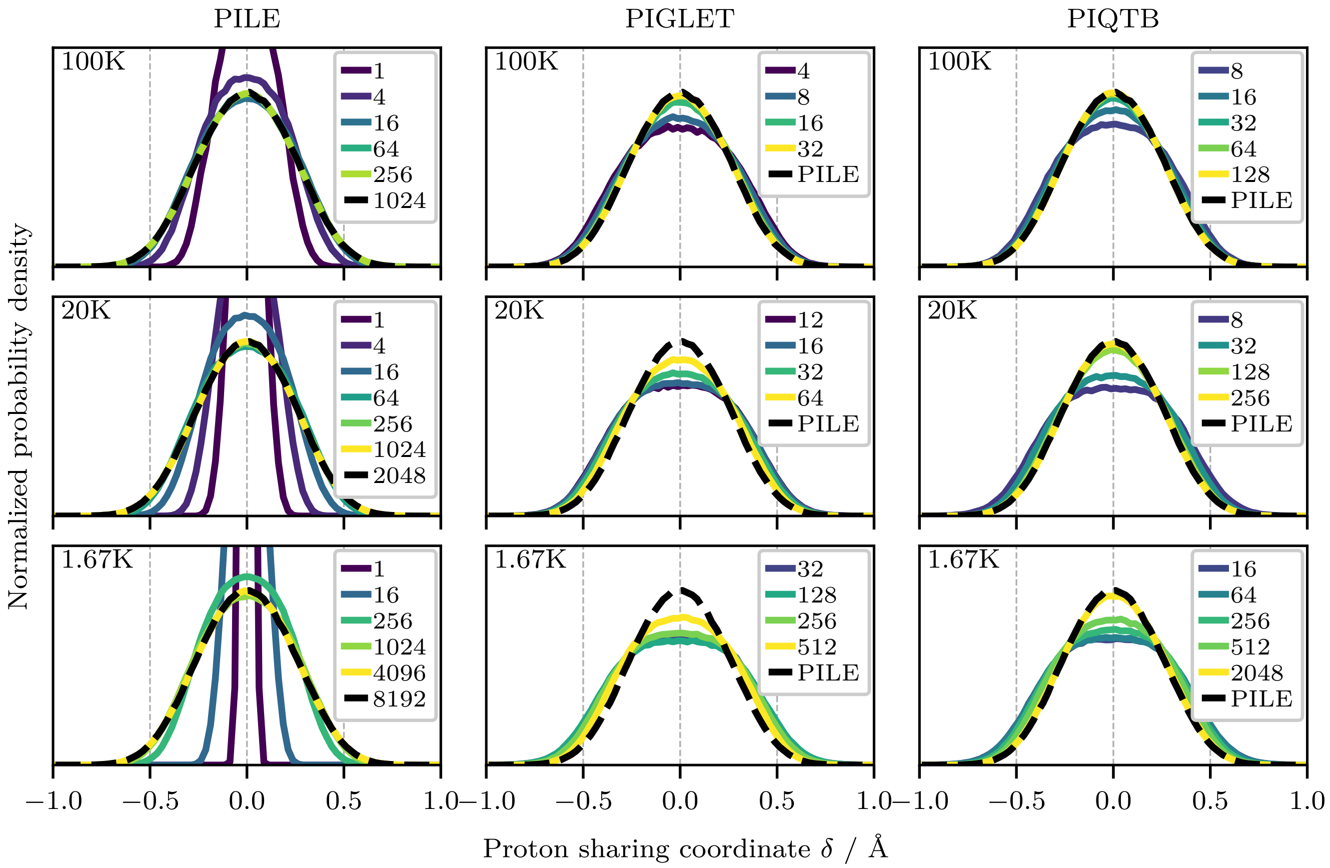


Figure 3. Distribution functions of the proton sharing coordinate, $\delta = r_{O_1H} - r_{O_2H}$ with $r_{O_1H}$ and $r_{O_2H}$ being the distance between the shared proton and oxygen $O_1$ and $O_2$, respectively, for different numbers of replicas $P$ at $T$ =100, 20 and 1.67 K for the PILE (left), PIGLET (middle) and PIQTB (right) thermostats (where in the middle and right panels the dashed black lines correspond to the PILE reference data obtained with the largest $P$ value).

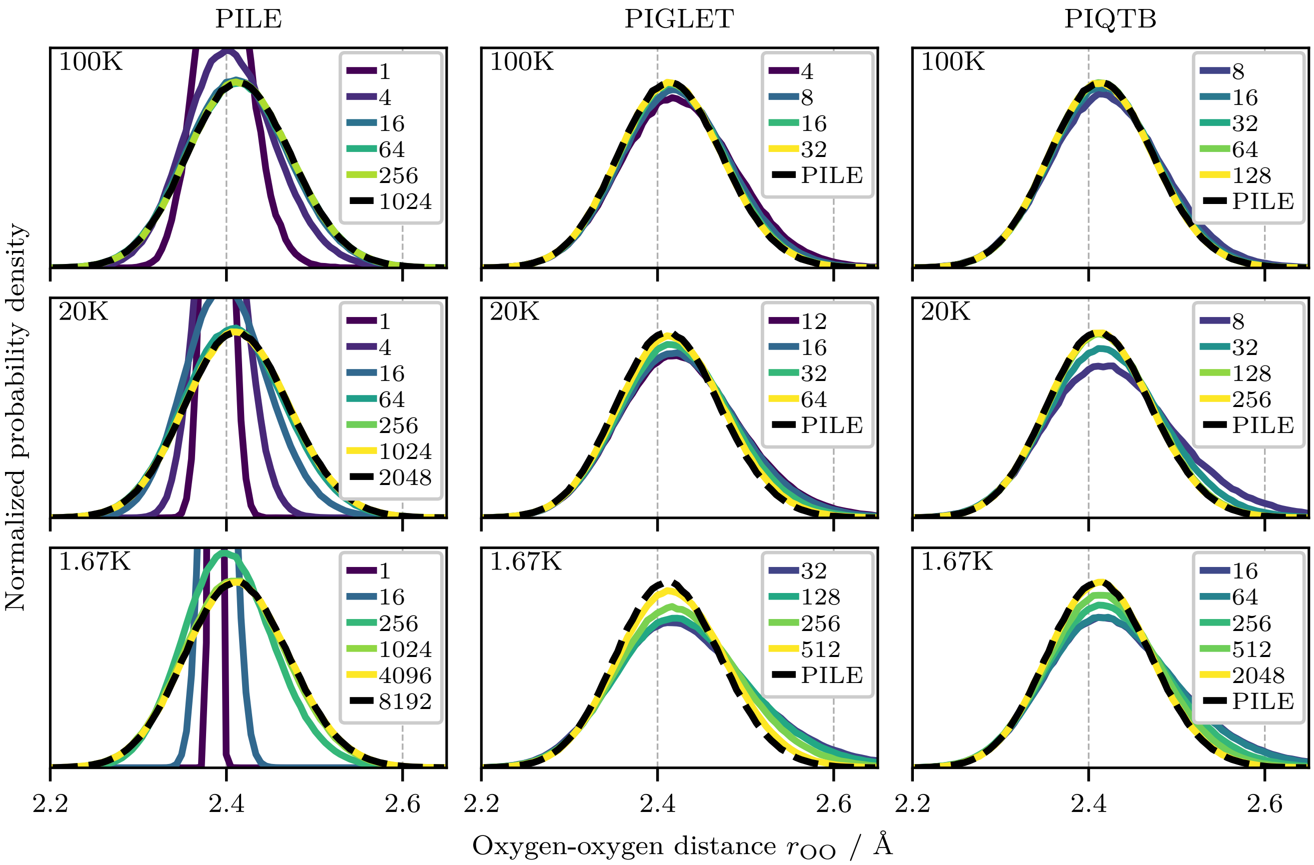


Figure 4. Distribution functions of the oxygen-oxygen distance, $r_{OO}$, for different numbers of replicas $P$ at $T$ =100, 20 and 1.67 K for the PILE (left), PIGLET (middle) and PIQTB (right) thermostats (where in the middle and right panels the dashed black lines correspond to the PILE reference data obtained with the largest $P$ value).

## III. SUPPORTING ANALYSIS ON NUCLEAR DELOCALIZATION PROPERTIES

In Fig. 5, the convergence of the radii of gyration of the different atoms in the Zundel cation at 100 and 20 K are depicted in order to complement the discussion in Sec. IV.C of the main text.

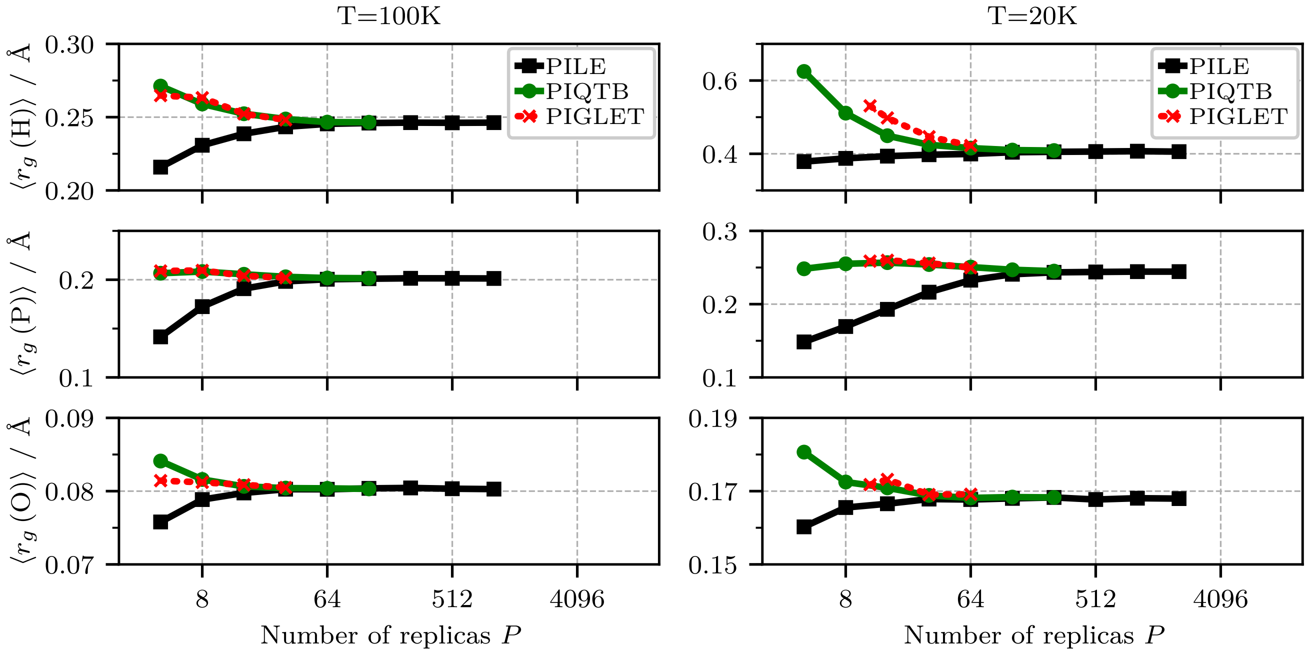


Figure 5. Convergence of the radius of gyration, $\langle r_g \rangle$, with respect to the number of replicas $P$ for the dangling hydrogen atoms (top), the shared proton (middle), and the oxygen atoms (bottom) at 100 and 20 K as obtained using the PILE (black squares), PIGLET (red crosses) and PIQTB (green circles) thermostats.


[1] H. Dammak, Y. Chalopin, M. Laroche, M. Hayoun, J.-J. Greffet, *Phys. Rev. Lett.* **2009**, *103*, 190601.
[2] F. Brieuc, H. Dammak, M. Hayoun, *J. Chem. Theory Comput.* **2016**, *12*, 1351–1359.
[3] M. Ceriotti, D. E. Manolopoulos, *Phys. Rev. Lett.* **2012**, *109*, 100604.
[4] M. Ceriotti, G. Bussi, M. Parrinello, *Phys. Rev. Lett.* **2009**, *103*, 030603.
[5] CP2k Developers Team, **2018**, www.cp2k.org.
[6] J. Hutter, M. Iannuzzi, F. Schiffmann, J. VandeVondele, *WIREs: Comput. Mol. Sci.* **2014**, *4*, 15–25.
[7] M. Ceriotti, M. Parrinello, T. E. Markland, D. E. Manolopoulos, *J. Chem. Phys.* **2010**, *133*, 124104.
[8] J.-L. Barrat, D. Rodney, *J. Stat. Phys.* **2011**, *144*, 679–689.
